# Supplementary material for: What really matters for person re-identification? A Mixture-of-Experts Framework for Semantic Attribute Importance
Source: arXiv:2512.08697 source file (2025-12-09)
Supplement: Supplementary file 1 [file glm_results_rank-1.tex]

\begin{table}
\caption{GLM Regression Results}
\label{tab:glm_results}
\begin{tabular}{lrrrrrr}
\toprule
 & Coef. & Std.Err. & z & P>|z| & [0.025 & 0.975] \\
\midrule
Intercept & 91.743898 & 0.078717 & 1165.493660 & 0.000000 & 91.589616 & 91.898180 \\
backpack & 0.276683 & 0.211773 & 1.306512 & 0.191379 & -0.138383 & 0.691750 \\
bag & -0.023317 & 0.211773 & -0.110102 & 0.912329 & -0.438383 & 0.391750 \\
handbag & 0.376683 & 0.211773 & 1.778716 & 0.075286 & -0.038383 & 0.791750 \\
hat & -0.223317 & 0.211773 & -1.054511 & 0.291649 & -0.638383 & 0.191750 \\
boots & 0.186289 & 0.186325 & 0.999807 & 0.317404 & -0.178901 & 0.551478 \\
shoecolour & -0.113711 & 0.186325 & -0.610286 & 0.541672 & -0.478901 & 0.251478 \\
top & 0.215525 & 0.166400 & 1.295227 & 0.195242 & -0.110612 & 0.541663 \\
gender & 0.332206 & 0.187787 & 1.769058 & 0.076884 & -0.035850 & 0.700262 \\
downcolour & 0.213594 & 0.149965 & 1.424295 & 0.154361 & -0.080332 & 0.507520 \\
upcolour & 0.039361 & 0.167414 & 0.235112 & 0.814122 & -0.288765 & 0.367487 \\
\bottomrule
\end{tabular}
\end{table}
