# Supplementary material for: What really matters for person re-identification? A Mixture-of-Experts Framework for Semantic Attribute Importance
Source: arXiv:2512.08697 source file (2025-12-09)
Supplement: Supplementary file 2 [file ttest_results_table_rank-1.tex]

\begin{table}
\caption{t-Test Results for Binary Attributes vs mAP}
\label{tab:ttest_results}
\begin{tabular}{lrrrr}
\toprule
Feature & t-stat & p-value & Cohen's d & Significance \\
\midrule
backpack & -2.471 & 0.049 & 1.616 & * \\
bag & -1.918 & 0.106 & 1.280 &  \\
handbag & -2.655 & 0.039 & 1.749 & * \\
hat & -1.577 & 0.170 & 1.090 &  \\
boots & -1.289 & 0.246 & 0.841 &  \\
shoecolour & -0.911 & 0.400 & 0.620 &  \\
top & -1.427 & 0.219 & 1.081 &  \\
gender & -0.753 & 0.588 & 1.663 &  \\
downcolour & -1.551 & 0.188 & 1.180 &  \\
upcolour & -1.825 & 0.118 & 1.182 &  \\
\bottomrule
\end{tabular}
\end{table}
