# Supplementary material for: What really matters for person re-identification? A Mixture-of-Experts Framework for Semantic Attribute Importance
Source: arXiv:2512.08697 source file (2025-12-09)
Supplement: Supplementary file 3 [file glm_results_rank-1.tex]

\begin{table}
\caption{GLM Regression Results}
\label{tab:glm_results}
\begin{tabular}{lrrrrrr}
\toprule
 & Coef. & Std.Err. & z & P>|z| & [0.025 & 0.975] \\
\midrule
Intercept & 94.912251 & 0.102073 & 929.850145 & 0.000000 & 94.712192 & 95.112310 \\
gender & -0.093235 & 0.294719 & -0.316350 & 0.751737 & -0.670873 & 0.484404 \\
hair & 0.406765 & 0.294719 & 1.380180 & 0.167531 & -0.170873 & 0.984404 \\
age & 0.706765 & 0.294719 & 2.398099 & 0.016480 & 0.129127 & 1.284404 \\
hat & -0.104415 & 0.309831 & -0.337006 & 0.736112 & -0.711674 & 0.502843 \\
backpack & 0.095585 & 0.309831 & 0.308506 & 0.757697 & -0.511674 & 0.702843 \\
bag & 0.495585 & 0.309831 & 1.599531 & 0.109703 & -0.111674 & 1.102843 \\
handbag & 0.095585 & 0.309831 & 0.308506 & 0.757697 & -0.511674 & 0.702843 \\
up & 0.277515 & 0.265555 & 1.045036 & 0.296006 & -0.242964 & 0.797994 \\
upcolour & 0.377515 & 0.265555 & 1.421605 & 0.155141 & -0.142964 & 0.897994 \\
down & 0.164260 & 0.295174 & 0.556486 & 0.577878 & -0.414270 & 0.742791 \\
downcolour & 0.764260 & 0.295174 & 2.589184 & 0.009620 & 0.185730 & 1.342791 \\
clothes & 0.264260 & 0.295174 & 0.895269 & 0.370643 & -0.314270 & 0.842791 \\
\bottomrule
\end{tabular}
\end{table}
