# Supplementary material for: What really matters for person re-identification? A Mixture-of-Experts Framework for Semantic Attribute Importance
Source: arXiv:2512.08697 source file (2025-12-09)
Supplement: Supplementary file 4 [file ttest_results_table_rank-1.tex]

\begin{table}
\caption{t-Test Results for Binary Attributes vs mAP}
\label{tab:ttest_results}
\begin{tabular}{lrrrr}
\toprule
Feature & t-stat & p-value & Cohen's d & Significance \\
\midrule
gender & -3.760 & 0.003 & 1.728 & ** \\
hair & -4.392 & 0.001 & 1.922 & *** \\
age & -4.822 & 0.000 & 2.054 & *** \\
hat & -2.264 & 0.051 & 1.153 &  \\
backpack & -2.437 & 0.037 & 1.207 & * \\
bag & -2.814 & 0.018 & 1.319 & * \\
handbag & -2.437 & 0.037 & 1.207 & * \\
up & -2.735 & 0.022 & 1.319 & * \\
upcolour & -2.830 & 0.018 & 1.348 & * \\
down & -3.599 & 0.006 & 1.831 & ** \\
downcolour & -4.560 & 0.001 & 2.099 & *** \\
clothes & -3.742 & 0.005 & 1.872 & ** \\
\bottomrule
\end{tabular}
\end{table}
